# Supplementary material for: Inverse Dynamic Games Based on Maximum Entropy Inverse Reinforcement Learning
Source: arXiv:1911.07503 source file (2020-07-24)
Supplement: Supplementary file 1 [file appendix.tex]

\section{Approximation of the Maximum Entropy Distribution}\label{app:Levine}

The integral in the denominator of \eqref{eq:global_Wahrscheinlichkeitsdichte2} and \eqref{eq:WahrscheinlichkeitTrajektorieSpieleriOpenloop} is computationally intractable and therefore, an approximation is necessary. This may be achieved by replacing the integral with a sum over several trajectory samples which are either already given \cite{kalakrishnan_learning_2013} or determined in each iteration from a forward optimal control or dynamic game solution with current cost function parameter candidates \cite{aghasadeghi_maximum_2011}. In this paper, we follow the approach which was applied in \cite{levine_continuous_2012} for the single-player case. Hence, we choose to approximate the integral and therewith, the probability density functions by applying a local approximation of each player's accumulated costs.
We exemplarily show the steps for the approximation of \eqref{eq:WahrscheinlichkeitTrajektorieSpieleriOpenloop} corresponding to the density function used for identification in Nash dynamic games. The approximation of \eqref{eq:global_Wahrscheinlichkeitsdichte2} for cooperative games is analogous.

For any control trajectory $\tilde{\underline{\m{u}}}_i$ and the resulting state trajectories $\tilde{\underline{\m{x}}}$, the cost function $J_i$ is approximated by means of a Taylor series expansion around the expert controls $\m{u}_{i,E_l}$ corresponding to the trajectory $\zeta_{E_l}$. This results in
\begin{equation}\label{eq:TaylorKostenMehrspieler}
\begin{split}
	J_i\left(  \tilde{\underline{\m{u}}}_i \right)&\approx J_i\left(  \underline{\m{u}}_{i,E_l} \right) + \left(\tilde{\underline{\m{u}}}_i - \m{\underline{u}}_{i,E_l} \right)^\top \underbrace{\left.\frac{\text{d}J_i}{\text{d}\tilde{\underline{\m{u}}}_i}\right|_{\tilde{\underline{\m{u}}}_i= \m{\underline{u}}_{i,E_l}}}_{=:\textstyle\m{g}_i} ... \\
	&+ \frac{1}{2} \left(\tilde{\underline{\m{u}}}_i - \m{\underline{u}}_{i,E_l}\right)^\top \underbrace{\left.\frac{\text{d}^2 J_i}{\text{d}\tilde{\underline{\m{u}}}_i^2}\right|_{\tilde{\underline{\m{u}}}_i= \m{\underline{u}}_{i,E_l}}}_{=: \textstyle\m{G}_i} \left(\tilde{\underline{\m{u}}}_i - \m{\underline{u}}_{i,E_l} \right),
\end{split}
\end{equation}
The gradient $\m{g}_i$ and the Hessian $\m{G}_i$ corresponding to player $i$ are defined as
\begin{align}
		\m{g}_{i,E_l}{}\coloneqq{}&\left.\frac{\partial J_i}{\partial \tilde{\underline{\m{u}}_i}} +\frac{\partial \underline{\m{x}}}{\partial \tilde{\underline{\m{u}}_i}}^\top\frac{\partial J_i}{\partial \tilde{\underline{\m{x}}}}\right\vert_{\subalign{\tilde{\underline{\m{u}}}_i\!\,&=\,\underline{\m{u}}_{i,E_l}\\ \vspace{3mm} \tilde{\underline{\m{x}}}\,&=\,\underline{\m{x}}_{E_l}}},\label{g_H}
\end{align}
and
\begin{align}
	\m{G}_{i,E_l}{}\coloneqq{}&\left.
	{\frac{\partial^2 J_i}{\partial \tilde{\m{\underline{u}}}_i^2}}
	+{\frac{\partial \m{\underline{x}}}{\partial \tilde{\m{\underline{u}}}_i}^\top}{\frac{\partial^2 J_i}{\partial \tilde{\m{\underline{x}}}^2}}
	{\frac{\partial \m{\underline{x}}}{\partial \tilde{\m{\underline{u}}}_i}} +  \frac{\partial^2\underline{\m{x}}}{\partial\tilde{\m{\underline{u}}}_i^2}
	\right\vert_{\subalign{\tilde{\underline{\m{u}}_i}\!\,&=\,\underline{\m{u}}_{i,E_l}\\ \vspace{3mm} \tilde{\underline{\m{x}}}\,&=\,\underline{\m{x}}_{E_l}}},
	\label{H}
\end{align}
where 
\begin{align*}
\frac{\partial J_i}{\partial \tilde{\underline{\m{u}}_i}} &\in \mathbb{R}^{m_i k_E \times 1} & 
\frac{\partial J_i}{\partial \tilde{\underline{\m{x}}}} &\in \mathbb{R}^{n k_E \times 1} \\
\frac{\partial^2 J_i}{\partial \tilde{\m{\underline{u}}}_i^2} &\in \mathbb{R}^{m_i k_E \times m_i k_E} &
\frac{\partial^2 J_i}{\partial \tilde{\m{\underline{x}}}^2} &\in \mathbb{R}^{n k_E \times nk_E}.
\end{align*}
Following \cite{levine_continuous_2012}, we set $\frac{\partial^2 \m{\underline{x}}}{\partial \m{\underline{u}}^2}=\m{0}$, which corresponds to linearizing the system dynamics in each time step.
The term 
\begin{equation}\label{dxdu_matrix}
{\frac{\partial \m{\underline{x}}}{\partial \tilde{\m{\underline{u}}}_i}^\top}:=\begin{bmatrix}
\m{D}_{1,1} & \dots & \m{D}_{1,T} \\ \vdots & \ddots & \vdots \\ \m{D}_{T,1} & \dots & \m{D}_{T,T}
\end{bmatrix}
\end{equation}
denotes the influence of the controls $\m{u}_i$ on the state $\m{x}$ at each time step $k \in \mathbb{K}$. Therefore, the block matrices within are given by
\begin{equation}
\setlength{\nulldelimiterspace}{0pt}
\m{D}_{k_1,k_2}=\left\{\begin{IEEEeqnarraybox}[\relax][c]{l?s}
\frac{\partial \m{x}^{(k+1)}}{\partial\m{u}_i^{(k)}}^\top\bigg|_{k=k_1},&for $k_2 = k_1+1$\\
\left.\m{D}_{k_1,k_2-1}\frac{\partial \m{x}^{(k+1)}}{\partial\m{x}^{(k)}}^\top\right|_{k=k_2-1},&for $k_2 > k_1+1$\\
\m{0},& else,%
\end{IEEEeqnarraybox}\right. ,
\end{equation}
where ${\m{D}_{k_1,k_2}=\frac{\partial \m{x}^{\left(k_2\right)}}{\partial \m{u}_i^{\left(k_1\right)}}^\top}$, ${k_1,k_2\in \mathbb{K}}$, are blocks of dimension $m_i\times n$ representing the influence of the player $i$'s control at time step $k_1$ on the states at time step $k_2$. These partial derivatives are part of the numerical solution of the initial value problem which approximates the next state. The matrix $\m{D}$ employs the partial derivatives with respect to $\m{u}$ in each time step for the whole corresponding time interval between two time steps. Contrary to this approach, we propose a modification of the matrix $\m{D}$ in order to improve the approximation. Inspired by the trapezoid method for solving initial value problems \cite[Section 6.5]{Epperson2013}, we approximate the effect of $\m{u}^{(k_1)}$ at $k_1$ on $\m{x}^{(k_2)}$ by means of 
\begin{equation}\label{D_tilde}
\m{\tilde{D}}_{k_1, k_2}\coloneqq\frac{1}{2}\left(\frac{\partial \m{x}^{(k_2)}}{\partial \m{u}^{(k_1)}}+\frac{\partial \m{x}^{(k_2+1)}}{\partial \m{u}^{(k_1)}}\right)^\top.
\end{equation}

The modified matrix $\m{\tilde{D}}$ takes in to account the effect of the control value $\m{u}^{(k_1)}$ on the interval of $\boldsymbol{x}^{(k_2)}$ until $\boldsymbol{x}^{(k_2+1)}$ and yields a better approximation of the system dynamics.

With known expert trajectories $\zeta_E$, it is possible to determine the gradient $\m{g}_i$ and the Hessian $\m{G}_i$ as a function of $\m{\theta}_i$, i.e. $\m{g}_i=\m{g}_i(\m{\theta}_i)$, $\m{G}_i=\m{G}_i(\m{\theta}_i)$.

By reformulating \eqref{eq:WahrscheinlichkeitTrajektorieSpieleriOpenloop} using the Taylor series based approximation \eqref{eq:TaylorKostenMehrspieler} of the cost function and considering that the trajectory $\zeta$ is uniquely defined by the controls $\underline{\m{u}}_i$ and the initial state $\m{x}^{(1)}$, we obtain
\begin{align}
\mathrm{p}\left(\left.\underline{\m{u}}_{i,E_l}\right|\m{x}^{(1)},\m{\theta}_i\right)=\frac{\text{e}^{-J_i\left(\left.\underline{\m{u}}_{i,E_l}\right|\m{x}^{(1)},\m{\theta}_i\right)}}{\displaystyle{\int_{-\infty}^{\infty}\text{e}^{-J_i\left(\left.\tilde{\underline{\m{u}}}_i\right|\m{x}^{(1)},\m{\theta}_i\right)}}~\text{d}\tilde{\underline{\m{u}}}_i}\nonumber\\	\hspace{1.5cm}\approx \text{e}^{\left(-\frac{1}{2}\m{g}_{E_l}^\top\m{G}_{E_l}^{-1}\m{g}_{E_l}\right)}\det\left(\m{G}_{E_l}\right)^{\frac{1}{2}}(2\pi)^{-\frac{\text{dim}(\underline{\m{u}}_i)}{2}}\nonumber.
\end{align}
